# Supplementary material for: Optimal Behavior Prior: Data-Efficient Human Models for Improved Human-AI Collaboration
Source: arXiv:2211.01602 source file (2022-11-19)
Supplement: Supplementary file 1 [file 70-appendix.tex]

\section{Appendix}

Our codebase can be found \href{https://drive.google.com/drive/folders/1FxVYE7qhXOeFSuNGbTzaTuzF8Uz2eL-D?usp=sharing}{here}. Code assets that we build off of, are: gym-minigrid's code \citep{chevalier2018minigrid} (Apache License 2.0), Decision Transformer's code \citep{chen_decision_2021} (MIT License), and D4RL's code \citep{fu2020d4rl} (Apache License 2.0).

\orrp{For camera ready, replace \texttt{\textbackslash section\{Appendix \}} with \texttt{\textbackslash appendix}, and then promote all sections (subsection to section, subsubsection to subsection, etc.). Not doing this right now because then our references to the submitted paper would change.}

\subsection{Training regimes details}\label{appx:training_regimes_deets}

Each batch is made of many randomly sampled trajectory snippets. Across the tasks depicted in \Cref{fig:tasks}, for each snippet $\tau_{t:t+k}$ we describe the input masking and predicted outputs in detail:

\begin{itemize}
    \item \textbf{Behavioral Cloning.} Select $i \in [0, k]$ uniformly. Feed $s_{t:t+i}, a_{t:t+i-1}$ to the network (include no actions if $i=0$), with all other tokens masked out. Have the network only predict the next missing action $a_i$.
    % \item \textbf{Next action completion.} Uniformly at random, sample from the dataset an action to predict $a_t$. Give the network the context $s_{t-k}, \dots, s_t, a_{t-k}, \dots, a_{t}$, with $a_t$ masked out. If the action is at the beginning of a trajectory, mask the all tokens in the extra context length. This is equivalent to standard behavior cloning training. 
    \item \textbf{Goal-Conditioned imitation.} Same as BC, but $s_{t+k}$ is always unmasked.
    \item \textbf{Reward-Conditioned imitation (Offline-RL).} Same as BC, but return-to-go $\hat{R}_t$ is always unmasked.
    \item \textbf{Waypoint-Conditioned imitation.} Same as BC, but a subset of intermediate states are always unmasked as waypoints or subgoals. %$s_{t_1}, \ldots s_{t_n}$ are always unmasked.
    \item \textbf{Future inference.} 
    % Uniformly at random, sample a sequence of length $k$ from all data. 
    % Select $t \in [0, k]$ uniformly. Mask the end of the trajectory $\{a_t, s_{t+1}, a_{t+1}, \ldots, a_w, s_w\}$ where $w$ is the last index of the context window. 
    Same as BC, but the model is trained to predict all future states and actions, rather than only the next missing action.
    % For each sequence, we generate $T$ training sequences $\tau_{i=1}^T$. For training sequence $\tau_i$, we mask the end of the trajectory $\{(a_t, s_{t+1}, a_{t+1}, \ldots, a_T, s_T\}$.
    \item \textbf{Past inference.} Select $i \in [1, k]$ uniformly. Feed $s_{t+i:t+k}, a_{t+i:t+k}$ to the network, with all other tokens masked out. Have the network predict all previous states and actions $s_{t:t+i-1}, a_{t:t+i-1}$.
    %We condition the model on a final state $s_{T-1}$. 
    %We roll out predicted actions \emph{and} states in reverse: for each timestep $t \in (T-2),\ldots, 0$, first sampling $a_t = \arg\max_{a_{t}'} p(a_{t}' \mid s_T, a_{T-1}, s_{T-1}, \ldots, s_{t+1})$ . Since we do not typically have access to an inverse dynamics model, we query the model for the state at time $t$ given the future trajectory: $s_t = \arg\max_{s_{t}'} p(s_{t}' \mid s_T, a_{T-1}, s_{T-1}, \ldots, s_{t+1}, a_{t})$. \MicahComment{make probability notation consistent across paper}\MicahComment{give more details about waypoinging in gridworld later}
    \item \textbf{Forward dynamics.} Select $i \in [0, k-1]$ uniformly. Give the network the current state and action $s_{t+i}, a_{t+i}$, and have it predict the next state $s_{t+i+1}$. In theory, this could enable to handle also non-Markovian dynamics (we did not test this).
    \item \textbf{Inverse dynamics.} Select $i \in [1, k]$ uniformly. Give the network the current state and previous action $s_{t+i}, a_{t+i-1}$, and have it predict the previous state $s_{t+i-1}$.
    \item \textbf{All the above (ALL).} Randomly select one of the above masking schemes and apply it to the current sequence. This is a simple way of performing multi-task training.
    \item \textbf{Random masking (RND).} 
    % Uniformly at random, sample a sequence of length $k$ from the data. 
    As we mention in \cref{sec:masking_schemes}, for each trajectory snippet, first, a masking probability $\pmask \in [0,1]$ is sampled uniformly at random; then each state and action token is masked with probability $\pmask$; lastly, the first RTG token is masked with probability $1/2$ and subsequent RTG tokens are masked always (see \Cref{sec:rnd-masking} for additional details). Randomly using the return-to-go in this fashion enables the model to perform both reward-conditioned and non-reward-conditioned tasks at inference time.
\end{itemize}

\subsection{Random masking scheme details}\label{sec:rnd-masking}

Given the significance of \iref{tr:random} in our work, let us take a closer look at the choices made in constructing this masking scheme.

A straightforward randomized masking would be to simply mask each of the state and action tokens with some fixed probability (in other words, fixing $\pmask=p$ for some constant $p$ rather than sampling it from $[0,1]$). Indeed, this is a common masking scheme in NLP uses of BERT. However, in this scheme, the \emph{number of masked tokens} is distributed as $\Binomial(k,p)$ where $k$ is the context length. Then, the probability of almost fully-masked (or fully-unmasking) a trajectory snipped is exponentially small in $k$. This is an issue for us, since there are many meaningful tasks that require most tokens to be masked (past prediction) or unmasked (behavior cloning).

Our alternative distribution resolves this problem. In this distribution (described in the first paragraph of this subsection), the \emph{number of masked tokens} is uniform in $[0,k]$.\footnote{See, for example, \url{https://math.stackexchange.com/q/282347}.} In particular the tails are not exponentially small in $k$. Empirically, we found that this distribution works much better than the straightforward distribution described in the previous paragraph.

\subsection{Model architecture details}\label{appx:model_details}

% \todo{discuss embedding sizes and other model details that are diff from transformer, stacking, how we only ever condition on return-to-go at timestep 0}

\prg{Input stacking.} %The main bottleneck for transformer models is usually the input sequence length: computational cost grows $O(n^2)$. In the context of decision processes, stacking state, action, and reward inputs would trivially enable to reduce the number of sequential inputs to the transformer by $3$ times relative to DT \citep{chen_decision_2021} and by $(N+M+1)$ times relative to Trajectory Transformer (where $N,M$ are the dimensionality of the state and action spaces) \citep{janner_reinforcement_2021}.

An important hyperparameter for transformer models is what dimension to use self-attention over. Previous work applies it across states, actions, and rewards as separate tokens (or even individual state and action dimensions) \citep{chen_decision_2021, janner_reinforcement_2021}; this can increase the effective sequence length that we would need to input a trajectory snippet of length $k$: for example if treating states, actions, and rewards separately (have self-attention act on each independently), the sequence length would be $3k$. While this is not an issue for the short context windows we use in our experiments, this seems wasteful: the main bottleneck for transformer models is usually the computational cost of self-attention, which scales quadratically in the sequence length. 

To obviate this problem, we stack states, actions, and rewards for each timestep, treating them as single inputs. This way, we are making self-attention happen only across timesteps, reducing the self-attention sequence length required to $k$. This also seems like a potentially advantageous inductive bias for improving performance. Though we did not test this systematically, preliminary experiments did show that input stacking sometimes reduced validation loss.

\prg{Return-to-go conditioning.} 

Unlike previous work that considers return-to-go conditioning \citep{chen_decision_2021}, we don't provide the model with many return-to-go tokens (one for each timestep). Providing just the first token should be sufficient for the model to interpret the return-to-go request (as, if necessary, the model can compute the remaining return to go in later steps). We found that this reduced overfitting for both \iref{tr:single} reward-conditioned training, or for \iref{tr:random} training. 

\prg{Positional/timestep encoding.} 

When conditioning on return-to-go tokens (i.e. for reward-conditioning), it is fundamental for the model to have information about what the time-horizon the specified return-to-go should be achieved by. To provide the model with this information \cite{chen_decision_2021} uses a ``timestep encoding'' instead of the standard positional encoding used in transformers: this consists of adding information to each input token which allows the model to identify to which trajectory-timestep such tokens correspond to. 

One large downside of this is that adding timestep information directly in this manner greatly increases the tendency of the model to overfit. To obviate this problem, we use positional encoding (which only provides the model with information about the relative position of each token within each trajectory snippet $\tau_{t:t+k}$). However, making the change to positional-encoding in isolation would remove trajectory-level timestep information from the return-to-go token (the problem that ``timestep encoding'' was introduced to solve). To address this, we change the form of the return-to-go token to a tuple containing return-to-go and the current timestep, and find this to work well in practice. 

%\MicahComment{We don't use timestep encoding anywhere in the paper as of right now, as it's not necessary for the minigrid bc of the horizon being short and also for mujoco (when not using RC)}

\subsection{Minigrid experiments details} \label{sec:doorkey-details}

Below we delineate some more details about our custom DoorKey minigrid environment.

\prg{Training dataset.} 

We train \fb{} models on training trajectories of sequence length $T=10$ from a noisy-rational agent \citep{ziebart_maximum_nodate} which takes the optimal action most of the time, but has some chance of making mistakes proportional to their sub-optimality. More specifically, the agent takes the optimal action with probability $a \sim p(a) \propto \exp (C(a))$ where $C(a)=1$ if the distance to the current goal (key or final goal) decreases, $-1$ if it increases, and $0$ otherwise.

\prg{Environment details.} 

The state and action spaces are both represented as discrete inputs: there are 4 actions, corresponding to the 4 possible movement directions (up, right, down, left); taking each action will move the agent in the corresponding direction unless 1) the agent is facing a wall, 2) the agent is facing the locked door without a key. Stepping on the key location tile picks up the key. The state is represented as two one-hot encoded position vectors---the agent position and the key position (which is equivalent to the agent position once the key has been picked up). Both agent and key position have 16 possible values, some of which are never seen in the data (e.g. the agent position coinciding with a wall location). Together, such vectors are sufficient to have full observability for the task---as seeing the key location coincide with the agent location informs the model that the agent is holding the key, and if the agent is holding the key it can open the locked door. Once the agent is holding the key, whether the door is open or closed is irrelevant.

Having the states and actions be discrete enables all model predictions to be done on a discrete space---which is particularly convenient as it enables the trained models to output any distribution over predicted states and actions, which can be easily visualized such as in \Cref{fig:state-viz}.

As the DoorKey environment have discrete actions and states, we use the softmax-cross-entropy loss over all predictions.

\prg{Fixing prediction inconsistencies.}

In backwards inference, we note that sometimes the predicted state at the previous timestep may not be consistent with the dynamics of the environment or the observed states. In cases where the prediction is inconsistent with environment dynamics, we re-sample the prediction (rejection sampling). In cases where the prediction is inconsistent with the observed variables, we simply return the trajectory even though it may not be consistent with the conditioned states, although rejection sampling could also have been performed here.

\prg{Hyperparameters.}

For each model and task, hyperparameters were obtained with a random-search method, which sweeped over batch sizes ($50, 100$), token embedding dimensions ($32$, $64$, or $128$), number of layers ($2$, $3$, or $4$), number of heads ($4$, $8$, or $16$), state loss re-scaling factors ($1$, $0.5$, or $0.1$), dropout ($0$ or $0.1$), and learning rates (selected log uniformly between $10^{-5}$ and $10^{-3}$). With number of layers, we refer to attention layers for transformers, and hidden layers for feedforward models. Optimal hyperparameter choice is reported in \Cref{tab:minigrid-hyperparams}.

Each model was trained using the Torch implementation of the Adam optimizer. Training was performed over $6000$ epochs with early stopping over the validation loss. Action:State loss indicates the relative re-scaling of the losses of actions and state predictions: we found it to sometimes be useful to offset the larger loss values of state predictions relative to action predictions (due to their larger dimensionality).

Each \iref{tr:finetune} model used the same hyperparameters as its corresponding \iref{tr:single} model, with the learning rate lowered to $5 \times 10^{-6}$ or $10^{-5}$, and the number of epochs to $500$--$6000$, depending on the task.

\begin{table}[]
    \centering
    
\begin{tabular}{P{2cm}|P{2cm}|c|c|c|c|c|c}
\hline 
Model & Training task & \shortstack{Batch \\ size} & \shortstack{Embed \\ dim.} & \shortstack{Layer \\ width} & \shortstack{Num. \\ layers} & \shortstack{Num. \\ heads} & \shortstack{Action:State \\ loss}\tabularnewline
\hline 
\hline 

 \multirow{2}{*}{\shortstack{\fb{} \\ \protect\iref{tr:single}}} & Behavior \newline Cloning & 250 & 32 & 128 & 2 & 4 & 1:0.1\tabularnewline

 & Reward \newline Conditioned & 50 & 32 & 128 & 3 & 4 & 1:1\tabularnewline

 & Goal \newline Conditioned & 250 & 128 & 128 & 3 & 8 & 1:1\tabularnewline

 & Waypoint \newline Conditioned & 250 & 128 & 128 & 3 & 8 & 1:1\tabularnewline

 & Past \newline Inference & 250 & 32 & 128 & 4 & 4 & 1:0.5\tabularnewline

 & Future \newline Inference & 250 & 128 & 32 & 2 & 4 & 1:0.5\tabularnewline

 & Forwards \newline Dynamics & 250 & 128 & 128 & 3 & 8 & 1:1\tabularnewline

 & Inverse \newline Dynamics & 50 & 128 & 128 & 3 & 8 & 1:0.5\tabularnewline
\hline 
\fb{} \newline \iref{tr:multi} & (All the above) & 250 & 32 & 128 & 3 & 4 & 1:1\tabularnewline
\hline 
\fb{} \newline \iref{tr:random} & - & 100 & 128 & 128 & 2 & 8 & 1:1\tabularnewline
\hline 
Decision \newline Transformer & Behavior \newline Cloning & 250 & 32 & 128 & 3 & 8 & 1:1\tabularnewline
\hline 
Decision \newline Transformer & Reward \newline Conditioned & 250 & 32 & 128 & 3 & 8 & 1:1\tabularnewline
\hline 
Multi-layer \newline Perceptron & Behavior \newline Cloning & 100 & 32 & 128 & 3 & - & 1:0.5\tabularnewline
\hline 
Multi-layer \newline Perceptron & Random \newline Masking & 250 & 32 & 128 & 3 & - & 1:0.5\tabularnewline
\hline 
\end{tabular}

    \caption{Hyperparameters chosen for each model and training task. In addition to the column headers, the sweep found the best learning rate to be $10^{-4}$ and dropout factor to be $0.1$, in all settings. \protect\iref{tr:finetune} models used the same hyperparameters as their corresponding \protect\iref{tr:single}, and are therefore omitted.}
    \label{tab:minigrid-hyperparams}
\end{table}

\prg{Computational cost.} 

Models were trained and evaluated on an on-premise server. The server has 256 AMD EPYC 7763 64-Core CPUs and 8 NVIDIA RTX A4000 GPUs. Running the experiments necessary to generate each of the heatmaps in the ``Detailed heatmaps'' section of \Cref{sec:additional-minigrid-exps} took approximately ten hours of compute. We were rarely able to fully utilize the server (since it is shared with other projects), but we estimate that with full parallelization the models and data for each heatmap would take roughly half an hour to generate.

\subsection{Additional minigrid experiments.}\label{sec:additional-minigrid-exps}

\prg{State-action distributions on MiniGrid}
% \label{sec:sa-viz}

We visualize the distribution of states and actions for trajectories sampled from the model, conditioned on the initial state (essentially, looking at the transition frequencies of BC-sampled trajectories). As seen in \Cref{fig:sa-viz}, the model learns to match the underlying distribution of trajectories of the agent (as can be verified by comparing to held-out data). 

\begin{figure*}[t]
    \centering
    \includegraphics[width=.4\textwidth]{images/sa_viz.pdf}
    \vskip -1.3em
    \caption{Distribution of states and actions for trajectories in the validation set, vs. trajectories sampled from the model, conditioned on the initial agent position (1,4) and key position (2,2).}
    \label{fig:sa-viz}
\end{figure*}

% \subsubsection{Detailed heatmaps}\label{sec:detailed-heatmaps}
\prg{Detailed heatmaps} 

We report below more validation-loss results from the minigrid experiments. This section expands on \Cref{fig:gridworld-valid-ranks500} by adding comparison to baseline models -- Decision Transformers (DT), and a Multi-layer Perceptron -- as well as varying the amount of data used to train each model (50, 1000, and the original 500). We see that notwithstanding the differences in dataset size, the trends and relative orderings of performance between models tend to stay the same.

All results are reported across six random seeds. All standard deviations are on the order of $0.01$, with the exception of about four cells (in each data regime) with especially high mean losses.

\MicahComment{add minor analysis of DT/NN results in appendix}

\prg{Decision Transformer with BC training.} 

When reporting performance for Behavior Cloning using Decision Transformer (DT), we are training a DT model without inputting return-to-go information at training time. This ensures that the model should be trying to directly imitate the expert, rather than trying to achieve any specific reward. This is also the case for \Cref{sec:maze-details}.

% \MicahComment{runs to verify our implemetnation of DT matches the original.} One exception is behavior cloning and offline-RL (behavior cloning), which seem to only lose a couple percentage points: this is likely an indication that in this environment, the reward information is not very informative

\begin{figure}[h!]
    \centering
    \includegraphics[width=0.9\columnwidth]{images/heatmaps/500_heatmap_normalized.png}
    \caption{Same as \Cref{fig:gridworld-valid-ranks500}, adding the last four rows that compare to baseline models.}
    \label{fig:gridworld-500-apx}
\end{figure}
\begin{figure}[h!]
    \centering
    \includegraphics[width=0.9\columnwidth]{images/heatmaps/500_heatmap.png}
    \caption{The raw loss values corresponding to \Cref{fig:gridworld-500-apx}.}
    \label{fig:gridworld-500-apx-raw}
\end{figure}
\begin{figure}[h!]
    \centering
    \includegraphics[width=0.9\columnwidth]{images/heatmaps/50_heatmap_normalized.png}
    \caption{\Cref{fig:gridworld-500-apx} when using a dataset of 50 trajectories instead of 500.}
    \label{fig:gridworld-50-apx}
\end{figure}
\begin{figure}[h!]
    \centering
    \includegraphics[width=0.9\columnwidth]{images/heatmaps/50_heatmap.png}
    \caption{The raw loss values corresponding to \Cref{fig:gridworld-50-apx}.}
    \label{fig:gridworld-50-apx-raw}
\end{figure}
\begin{figure}[h!]
    \centering
    \includegraphics[width=0.9\columnwidth]{images/heatmaps/1000_heatmap_normalized.png}
    \caption{\Cref{fig:gridworld-1000-apx} when using a dataset of 1000 trajectories instead of 500.}
    \label{fig:gridworld-1000-apx}
\end{figure}
\begin{figure}[h!]
    \centering
    \includegraphics[width=0.9\columnwidth]{images/heatmaps/1000_heatmap.png}
    \caption{The raw loss values corresponding to \Cref{fig:gridworld-1000-apx}.}
    \label{fig:gridworld-1000-apx-raw}
\end{figure}

\MicahComment{ablation on stacking for DT?}

\subsection{Our Decision-GPT model} \label{sec:gpt-details}

To obtain our Decision-GPT model, we use a standard GPT architecture (i.e. using a transformer decoder with \textit{causal} self-attention), but incorporate the return-to-go and positional encoding design choices we used for \fb{} models (which are described in \Cref{appx:model_details}). This is to form a improved baseline from a simple GPT model.

\MicahComment{maybe have another ablation where we consider showing all return-to-go tokens} 

\subsection{Maze2D experiments details} \label{sec:maze-details}

\prg{Choice of environment.} 

We initially set out to compare the performance of \fb{} on the same continuous control tasks used in \cite{chen_decision_2021}. However, after consulting with the authors of \cite{chen_decision_2021}, we decided not to use the classic Mujoco control environments and associated D4RL datasets~\cite{fu2020d4rl}. 

We list some of the issues with the D4RL datasets and classic control environments here: 1) given that the expert datasets were generated from Markovian policies and that these Mujoco environments are Markovian themselves, there is no direct reason for why sequence models should provide any benefit (although some benefit is observed in practice); 2) we noticed that completely overfitting a single trajectory with a MLP was sufficient for obtaining relatively good reward performance, indicating that such environments do not have enough inherent randomness to be a good indicator as to the generalization of trained policies -- which is what we ultimately care about.

We tried to address these points in modifying the Maze2D environment. By choosing an environment in which the start and goal location are randomized, overfitting is not a viable strategy for generalization: memorizing a single trajectory in this setup leads to extremely poor performance. 

As an additional detail, we modify the original environment reward to be dense, so that the reward at every timestep is given by the distance covered towards the goal.

See \Cref{fig:maze_env} for example initializations of the environment.

% \prg{Dataset generation.} We generate our data using D4RL's PD controller with a bug fixed. \MicahComment{move mention of the bug to the appendix, with description of it} The fact that such PD controller is non-Markovian is another advantage over using DT's environments: the datasets for their continuous control task were generated with agents parametrized with simple feed-forward networks, meaning that a sequence model is unnecessary to capture their behavior. We also modify the expert relative to what was used in \citep{fu2020d4rl}: we add random noise to the actions.

% \begin{figure}[h!]
%     \centering
%     \includegraphics[width=0.7\columnwidth]{images/maze_env.png}
%     \caption{}
%     \label{fig:maze_env}
% \end{figure}
 
\MicahComment{Maze dataset expert performance}

\begin{figure*}[t]
\noindent
\begin{minipage}[!t]{0.5\textwidth}
    \centering
    \includegraphics[width=0.7\columnwidth]{images/maze_env.png}
    \vskip -1.3em
\end{minipage}%
\hfill%
\begin{minipage}[!t]{0.5\textwidth}
    \centering
    \includegraphics[width=0.7\columnwidth]{images/maze_env2.png}
    \vskip -1.3em
\end{minipage}%
\caption{Examples of initializations in the Maze2D environment: the agent (in green) must navigate the environment to reach the goal (in red).}
\label{fig:maze_env}
\end{figure*}

\prg{Training details.} 

As the Maze2D environment has continuous actions and states, we use an L2 loss over all predictions. Each model was trained using the Torch implementation of the Adam optimizer. Training was performed for $1000$ epochs with early stopping over the evaluation reward. 

In reward-conditioned evaluation, choosing reasonable return-to-go (RTG) tokens on which to condition is non-trivial: asking for large reward in cases in which the goal is very close to the starting state leads to impossible-to-satisfy queries. Conversely, using the average reward as the goal return-to-go might be too conservative for easy initializations in which the point mass object can traverse most of the maze. To obviate this problem, we try to automatically determine what a reasonable RTG is at evaluation time using the following method: 1) reset the environment (leading to a random initial state); 2) find the trajectory in the dataset which has the most similar initial state (which also includes information about the goal location), and it's total reward $R$; 3) Condition on an RTG of $1.1 \times R$. We found this behave as intended qualitatively.

\prg{Hyperparameters.} 

For each model and task, hyperparameters were obtained with a random-search method, which sweeped over batch sizes ($50, 100, 200$), token embedding dimensions ($64, 128$), number of layers ($2$, $3$, or $4$), number of heads ($8$, $16$), state loss re-scaling factors ($1$, $0.5$, $0$), and learning rates (selected log uniformly between $10^{-5}$ and $10^{-3}$). With number of layers, we refer to attention layers for transformers, and hidden layers for feedforward models. 

Given that we found little difference between various hyperparameters across model types, the same set of hyperparameters was used across all conditions. The final hyperparameters are as follows: $10^{-4}$ learning rate, $100$ batch size, $128$ embedding dimension, $4$ layers, $16$ attention heads, and a state loss re-scaling factor of $1$ (equivalent to no re-scaling).

Similarly to the Minigrid experiments, each \iref{tr:finetune} model used the same hyperparameters as its corresponding \iref{tr:single} model, with the learning rate lowered to $8 \times 10^{-5}$, and the number of epochs lowered to $600$.

\MicahComment{more info on val loss != reward. describe goal-conditioned/waypoint}

\prg{Computational cost.} 

We used the same compute infrastructure for our Maze2D experiments as in the Minigrid experiments (described in \Cref{sec:doorkey-details}). A training run in Maze2D takes approximately 4 hours on our server, but more than 20 runs can be run in parallel. In total, running all runs for \Cref{table:maze_results} should take on the order of 10 hours when using our setup in parallel.
